# Supplementary material for: Derived Algebraic Cobordism
Source: arXiv:2203.12096 source file (2022-03-22)
Supplement: Supplementary file 1 [file appendix.tex]

\chapter{Supporting Materials}

This would be any supporting material not central to the dissertation.
For example:
\begin{itemize}
\item additional details of methodology and/or data;
\item diagrams of specialized equipment developed.;
\item copies of questionnaires and survey instruments.
\end{itemize}
